# Supplementary material for: Distributionally Robust Offline Reinforcement Learning with Linear Function Approximation
Source: arXiv:2209.06620 source file (2023-01-27)
Supplement: Supplementary file 1 [file appendix_2.tex]

\begin{proposition}
    \begin{align*}
    \lvert \iota_h(s,a)\rvert \le \newcoef \sqrt{c\cdot d\log (SK/\delta)} \lVert \phi(s,a)\rVert_{\Lambda_h^{-1}},
    \end{align*}
    for some absolute constant $c\ge 3$.
\end{proposition}

\begin{proof}
Note that $\widehat{\psi}_i \ll \psi_i$ since $\widehat{\psi}_i(s)$ is an unbiased estimator for $\psi_i(s)$ for every $s\in \gS$, we then have from Equation~\ref{eq:transition-3} and the fact that $\lvert \log(1+x)\rvert \le 2\lvert x\rvert$
\begin{align*}
    \lvert w_{h,i} - \widehat{w}_{h,i}\rvert &\le \maxb \{\beta_i\ln (1+\frac{\E_{\widehat{\psi}_{h,i}}[e^{-V_{h+1}(\spr)/\beta_i}] - \E_{\psi_{h,i}}[e^{-\widehat{V}_{h+1}(\spr)/\beta_i}]}{\E_{\psi_{h,i}}[e^{-\widehat{V}_{h+1}(\spr)/\beta_i}]})\} \\ 
    &\le \frac{2H}{\rho}\frac{\sum_{s\in \gS}\lvert \widehat{\psi}_{h,i}(s) - \psi_{h,i}(s)\rvert e^{-\widehat{V}_{h+1}(\spr)/\beta_i}}{\sum_{s\in \gS}\psi_{h,i}(s)e^{-\widehat{V}_{h+1}(\spr)/\beta_i}}\\
    &\le \frac{2H}{\rho}\max_{s\in \gS}\lvert \frac{\widehat{\psi}_i(s)}{\psi_i(s)} - 1 \rvert.
\end{align*}

% Note that for any $s\in \sS$,
% \begin{align*}
%     \lvert \frac{\widehat{\psi}_i(s)}{\psi_i(s)} \rvert &= \frac{\mathds{1}_i^{\top}\Lambda_h^{-1}[\sum_{\tau=1}^K \phi(s_h^{\tau}, a_h^{\tau})\mathds{1}(s_{h+1}^{\tau}=s)]}{\mathds{1}_i^{\top}\Lambda_h^{-1}[\sum_{\tau=1}^K \phi(s_h^{\tau}, a_h^{\tau})P_{h+1}(s\lvert s_{h}^{\tau}, a_{h}^{\tau})] + \lambda \mathds{1}_i^{\top}\Lambda_h^{-1}\psi}
% \end{align*}
Recall that 
\begin{align*}
    \lvert \widehat{\psi}_i(s) - \psi_i(s)\rvert &= \mathds{1}_i^{\top}\Lambda_h^{-1}[\sum_{\tau=1}^K \phi(s_h^{\tau}, a_h^{\tau})(\mathds{1}(s_{h+1}^{\tau}=s) - P_{h+1}(s\lvert s_{h}^{\tau}, a_{h}^{\tau}))] - \lambda \mathds{1}_i^{\top}\Lambda_h^{-1}\psi(s).
\end{align*}

Thus 
\begin{align*}
    \max_{s^{\prime}\in \gS} \lvert \frac{\widehat{\psi}_i(s)}{\psi_i(s)} - 1 \rvert &= \max_{s^{\prime}\in \gS} \frac{1}{\psi_i(s)}\lvert \widehat{\psi}_i(s) - \psi_i(s)\rvert\\
    &\le \max_{s^{\prime}\in \gS} \frac{1}{\underline{\psi}} \lvert \widehat{\psi}_i(s) - \psi_i(s)\rvert,
\end{align*}
where $\underline{\psi} = \min_{s^{\prime}}\psi_i(s^{\prime})$.

Thus we are in the position to control the error in the transition term,
\begin{align*}
    \phi(s,a)^{\top} (w_h-\widehat{w}_h) &= \sum_{i=1}^d \phi_i(s,a) (w_{h,i}-\widehat{w}_{h,i})\\
    &\le \frac{2H}{\rho} \sum_{i=1}^d \phi_i(s,a) \max_{s^{\prime}\in \gS} \lvert \frac{\widehat{\psi}_i(s^{\prime})}{\psi_i(s^{\prime})} - 1\rvert \\
    &\le \max_{s^{\prime}} \frac{2H}{\rho\underline{\psi}} \sum_{i=1}^d \phi_i(s,a)\left( \mathds{1}_i^{\top}\Lambda_h^{-1}[\sum_{\tau=1}^K \phi(s_h^{\tau}, a_h^{\tau})(\mathds{1}(s_{h+1}^{\tau}=s^{\prime}) - P_{h+1}(s^{\prime}\lvert s_{h}^{\tau}, a_{h}^{\tau}))] - \lambda \mathds{1}_i^{\top}\Lambda_h^{-1}\psi(s)\right)\\
    &\le \frac{2H}{\rho\underline{\psi}} \max_{s^{\prime}}\phi(s,a)^{\top}\Lambda_h^{-1}[\sum_{\tau=1}^K \phi(s_h^{\tau}, a_h^{\tau})(\mathds{1}(s_{h+1}^{\tau}=s^{\prime}) - P_{h+1}(s^{\prime}\lvert s_{h}^{\tau}, a_{h}^{\tau}))]\\
    &\quad + \max_{s^{\prime}}\frac{2H}{\rho\underline{\psi}} \phi(s,a)^{\top}\Lambda_h^{-1}\psi(s^{\prime}).
\end{align*}

\begin{align*}
    \lvert \phi(s,a)^{\top} (w_h-\widehat{w}_h)\rvert &\le \frac{2H}{\rho\underline{\psi}} \max_{s^{\prime}} \lVert \phi(s,a)\rVert_{\Lambda_h^{-1}} 
    \lVert \sum_{\tau=1}^K \phi(s_h^{\tau}, a_h^{\tau})(\mathds{1}(s_{h+1}^{\tau}=s^{\prime}) - P_{h+1}(s^{\prime}\lvert s_{h}^{\tau}, a_{h}^{\tau}))\rVert_{\Lambda_h^{-1}}\\
    &\quad + \max_{s^{\prime}}\frac{2H}{\rho\underline{\psi}}\lVert \phi(s,a)\rVert_{\Lambda_h^{-1}}\lVert \psi(s^{\prime})\rVert_{\Lambda_h^{-1}}
\end{align*}

For the second term 
\begin{align*}
    \lVert \psi(s^{\prime})\rVert_{\Lambda_h^{-1}} &= \sqrt{\psi(s^{\prime})^{\top}\Lambda_h^{-1}\psi(s^{\prime})}\\
    & = \lVert \Lambda_h^{-1}\rVert_{op}^{1/2}\cdot \lVert \psi(s^{\prime})\rVert\\
    &\le \sqrt{d/\lambda}.
\end{align*}

For the first term, we invoke Lemma~\ref{lm:self-normalized} and have the following holds with probability at least $1-\xi$,
\begin{align*}
    \max_{s^{\prime}}\lVert \sum_{\tau=1}^K \phi(s_h^{\tau}, a_h^{\tau})(\mathds{1}(s_{h+1}^{\tau}=s^{\prime}) - P_{h+1}(s^{\prime}\lvert s_{h}^{\tau}, a_{h}^{\tau}))\rVert_{\Lambda_h^{-1}} \le \highub.
\end{align*}

Thus 
\begin{align*}
    \lvert \phi(s,a)^{\top}(w_h-\widehat{w}_h)\rvert &\le \newcoef (\sqrt{\highub}+\sqrt{d/\lambda}) \lVert \phi(s,a)\rVert_{\Lambda_h^{-1}}\\
    &\le \newcoef \sqrt{c\cdot d\log (SK/\delta)} \lVert\phi(s,a)\rVert_{\Lambda_h^{-1}}.
\end{align*}

Finally we can conclude the bound for the Bellman error is 
\begin{align*}
    \lvert \iota_h(s,a)\rvert& = \lvert (\sB_h \hat{V}_{h+1})(s,a) -  (\hat{\sB}_h \hat{V}_{h+1})(s,a)\rvert\\
    &\le \beta_h \lVert \phi(s,a)\rVert_{\Lambda_h^{-1}},
\end{align*}
where $\beta_h = \newcoef \sqrt{c\cdot d\log (SK/\delta)}$ for some absolute constant $c\ge 3$.
\end{proof}
